# Supplementary material for: The asymptotic number of lattice zonotopes in a hypercube
Source: arXiv:2106.01005 source file (2023-02-11)
Supplement: Supplementary file 1 [file appendix.tex]

%    \interval is used to provide better spacing after a [ that
%    is used as a closing delimiter.

%    Notation for an expression evaluated at a particular condition. The
%    optional argument can be used to override automatic sizing of the
%    right vert bar, e.g. \eval[\biggr]{...}_{...}
\newcommand{\eval}[2][\right]{\relax
  \ifx#1\right\relax \left.\fi#2#1\rvert}

%    Enclose the argument in vert-bar delimiters:

%    Enclose the argument in double-vert-bar delimiters:

%\setcounter{tocdepth}{5}

\begin{document}

\title{The asymptotic number of zonotopes}

\author[T. Buffi{\`e}re]{Théophile Buffi{\`e}re}
\address{LAGA, Universit{\'e} Paris 13, Villetaneuse, France}
\email{buffiere@univ-paris13.fr}

%\date{Received on MONTH, YEAR}
%\issueinfo{VOL}{NUM}{MONTH}{YEAR}
%\doiinfo{10.1007/DOI-NUMBER}

\maketitle

\import{Parties/}{abstract.tex}

%\tableofcontents

\leavevmode\\
\leavevmode\\
Remarques: \\
Mathematics:\\
-polygonal lines\\
-trop d'emphase sur Mellin\\
-trop d'emphase sur Haymann -pas assez sur la méthode de de proba. \\
-décider de prendre ou non l'hypothèse de Riem\\

Ecritures:\\
-Prop 3, et lemma 4 pas assez détaillés\\
-Graphic illustration : Un zonotope au début, et  !\\
-refrences : complete the doi, and pages, les russes (funct anal appl) doivent diriger vers des trad anglaises.\\
-Noms, Ehrhart, Riemann mef !!!\\
- Toute l'écriture n'est pas claire, on veut un truc fluide.

Nouvelle strat:\\
-la combi n'est pas trop touchée, on garde. \\
-changer h admiss pour un truc plus matheux (prendre Stephen Melczer a la place de Gitten) ? \\
- Révision générale des démos, on fait des maths des vrais.  
Surtout détails maths de Eulerian et de H-admiss.\\
-Plus de relecture d'ortho (à froid, al f\'in)\\
-Idées claires sur Riemann hypo.\\

Trucs a faire:\\
- notations des theorem de l'intro a refaire\\
-Partie : analysis of the partition function (1. euler set 2. generating function equivalent), proof of the theorem,

\leavevmode\\
\leavevmode\\

\import{Parties/}{0introduction.tex}

\section{Class of zonotopes, combinatorial and probabilistic approach}\label{section_combi}
\import{Parties/}{1zonotopes_generating_function.tex}
\leavevmode\\

\section{Integral representation of Eulerian summation of coprimes}\label{section_eulerset}

The proof of Theorem \ref{theorem_1},  as it is the generalization of the result from \cite{Bureaux:polygons}, surprisingly follows the same framework, taking integral representation the integral through Mellin transform. It will lead to estimating the generating function near $\ttheta = 0$ using the utmost-left propagation of the integration contour of the transform. It turns out this method is possible thanks to the link between Eulerian polynomials and harmonic sums over primitive vectors. \medskip 

Let be $\aalpha \in \N^d$, $\un = (1,...,1)$, and $t > 0$, and denote $\text{int}(\R^d_{+})$ the interior of $\R^d_{+}$, the point in this section is to study the sum $S_{\aalpha} (e^{-t})$ that is

$$S_{\aalpha} (e^{-t}) = \sum_{\vv \in \P_{d+} \cap \text{int}(\R^d_{+})} \vv^{\aalpha} e^{ - t \un \cdot \vv} = \sum_{n = 1}^{+ \infty} \left( \sum_{\vv \in \P_{d+}\cap \text{int}(\R^d_{+}), \: \un \cdot \vv = n } \vv^{\aalpha} \right) e^{ - t n} $$

The partial sums over the primitive vectors with  {\color{red}L1-norm equals $n$} are denoted $S_n(\boldsymbol{\alpha})$. \medskip

\begin{rem}
As $\aalpha$ can have zero coordinate, the product $\vv^{\aalpha}$ is not always defined over $\P_{d+}$. the sum therefore covers non-zero-coordinated-integer. Yet the reader can see it as a sum over all elements of $\P_{d+}$ with the convention $\vv^{\aalpha} =0$ if and only if $\vv$ has a zero coordinate.   
\end{rem}

% \emph{dit pourquoi c'est cool Mellin, propriete de sortir les harmonique hors de l'integral. Réponse : je ne sais pas si c'est utile d'appuyer sur ça alors que les rapports disent que c'est vraiment facile d'utiliser Mellin, et je refais la propriété d'harmonique proprement avec Fubini plus loin.}
Before the proposition is given, we introduce the routinely used Mellin transform which is the transform that maps the exponential onto the Gamma function, that holds for all $s$, with $\Re(s) >0$:  

$$ \Gamma(s) = \int_{0}^{+ \infty} e^{-t} t^{s - 1} dt.$$

For a given function $f$ and two numbers $a <b$ such that $\underset{x \rightarrow 0}{\lim}f(x) = O(x^a)$ and  $\underset{x \rightarrow + \infty}{\lim}f(x) = O(x^b)$, for all $s$ with $a< \Re(s) <b$, the Mellin transform of $f$ is defined as:  

$$ \mathcal{M}\left[f\left(e^{-t}\right)\right](s) = \int_0^{+\infty} f\left(e^{-t}\right)t^{s-1}dt.$$

\begin{prop}\label{proposition_eulerian}

For $t>0$ and $s \in \C$ with $\Re(s) > \un \cdot \aalpha + d$:

 \begin{align}
     \mathcal{M}\left[ S_{\aalpha}(e^{-t}) \right](s) = \frac{1}{\zeta(s - \aalpha \cdot \un )} \mathcal{M}\left[ \frac { \prod_{i = 1}^{d}  A_{\alpha_i}(e^{-t})}{(1-e^{-t}) ^{\aalpha \cdot \un + d}}  \right](s) ,
 \end{align}
 
 where $A_{\alpha_i}$ denotes the Eulerian polynomial of degree $\alpha_i$.
\end{prop}

\medskip

Eulerian polynomials were first described by Euler \cite{Euler} while studying the series form of $\frac{y e^x}{1 - y e^x}$ \cite{Euler}. We denote $A_n$ the $n$-th Eulerian polynomial using the recursive definition:

$$\left\{ \begin{array}{l}
       A_0(y) = y,\text{ and} \\
       A_n(y) = \sum_{m= 0}^n A(n,m)y^{n-m}.
\end{array} \right.$$

Hence the first Eulerian polynomials are $A_1(y) = y, \; A_2(y) = y^2 + y,$ and $ A_3(y) = y^3 + 4 y^2 + y$. In particular, they satisfy the relation:

\begin{align}\label{eulerien_poly}
    \sum_{k=1}^\infty k^n y^{k}  &= \frac{ A_n (y)}{(1-y)^{n+1}}.
\end{align}

$$  
$$

\begin{lem}\label{lem_eulerian_sum_notation} 
For any complex number $y$ with $|y| < 1$, 
\begin{align}\label{relation_lem_eulerian}
    \sum_{k \geq 0} k^{\un \cdot \aalpha} S_{\aalpha} (y^k) =  \frac { \prod_{i = 1}^{d}  A_{\alpha_i}(y)}{(1-y) ^{\aalpha \cdot \un + d}} .
\end{align} 
\end{lem}

\begin{proof}

This relation relies on the partition $\N_+^r =\bigcup_{k \geq 0} \left\{ kp, p \in \mathbb{P}^r_+ \right\}$ and the definition of Eulerian polynomials. The left term can be written as: 

$$ \sum_{k \geq 0 } k^{\un \cdot \aalpha}  S_{\aalpha} (y^k) = \sum_{k \geq 0} \sum_{n \geq 1} \left(\sum_{\substack{ \vv \in \P_{d+} \cap \text{int}(\R^d_{+}) \\   \un \cdot \vv = n }}(k \vv)^{\aalpha}(y)^{k \un \cdot \vv} \right)$$ 

We recognize the set of summation to be the partition previously mentioned. Therefore, for $|y| < 1$, the term $\vv^{\aalpha} y^{\un \cdot \vv}$ implies the absolute convergence of this sum. Hence we can use Fubini-Tonelli theorem to inverse the sums, and the relation (\ref{eulerien_poly}) concludes the proof.

$$ \sum_{\substack{ \vv \in \N^d \cap \text{int}(\R^d_{+})} } \vv ^{\aalpha} y^{\vv}   = \prod_{i = 1}^{d} \left( \sum_{v_i \geq 1} v_i^{\alpha_i} y^{v_i} \right)  = \frac { \prod_{i = 1}^{d}  A_{\alpha_i}(y)}{(1-y) ^{\aalpha \cdot \un + d}}.  $$

\end{proof}

The $n^{th}$ Eulerian polynomial is of degree $n$ except for $A_0(y) = y$ and has no constant term which causes the degree of $\prod_{i = 1}^{d}  A_{\alpha_i}(y)$ to be no more than $\aalpha \cdot \un + d$ (which is achieved for $\aalpha = \textbf{0}$).  The $\aalpha$ of the sums under study in this paper are $\textbf{0}$, $(1,0..,0)$, and $(2,0...,0)$, and the product of polynomials, therefore equals $y^{d}$, $y^{d}$, or $y^{d+1}+ y^{d}$.\\

Note that $S_n(\boldsymbol{\alpha})$ is the sum of a power function over the primitive points contained in the hypersurface of the dilates of the $(r-1)$-dimensional standard simplex. It is noteworthy that the number of such points has been computed in \cite{DezaPournin:primitivepoint}.   \\

\begin{proof}[Proof of the proposition]

Under the condition $ \Re(s) > \aalpha \cdot \un + d - 1$, the Mellin transform of the sum (\ref{relation_lem_eulerian}) is defined. This condition ensures that {\tiny$\sup_{\Re(s) > \aalpha \cdot \un + d - 1} \sum_{k \geq 0} |\frac{k^{\aalpha \cdot \un}}{k^s} |$} is bounded, hence we can apply Fubini's theorem with the change of variable $t' = kt$  and we have:

$$ \int_0^{+\infty} \sum_{k \geq 0 } k^{\aalpha \cdot \un} S_{\aalpha}(e^{-kt}) t^{s-1} d t= \zeta(s-\aalpha\cdot \un) \: \mathcal{M}\left[ S_{\aalpha}(e^{-t}) \right](s).$$

These holomorphic functions being defined and equal on $\Re(s) > \aalpha \cdot \un + d - 1$, we can extend it to its meromorphic continuation on $\C$. We replace the left term using Lemma \ref{lem_eulerian_sum_notation} and get the proposition.

\end{proof}

The Mellin transform is widely used to estimate asymptotic behaviors using its correspondence with the poles of the transformed function, as we will do in next subsection (and as it is done in \cite{Bodini:polyomino} and \cite{Bureaux:polygons}).  Proposition \ref{proposition_eulerian} makes it possible to compute the asymptotic equivalent of any of the sums $S_{\aalpha}(y) $ near $y =1$.

\leavevmode\\

\section{Asymptotic analysis of the generating function}
\import{Parties/}{3analysis.tex}
\leavevmode\\

\section{Proof of the Theorem}\label{proof_main}
\import{Parties/}{5proof_theorem.tex}
\leavevmode\\

\section{Numerical elements about the speed of convergence to the asymptotic regime}\label{numerical_discu}
\import{Parties/}{6comments.tex}
\leavevmode\\

%\section{Appendices: H-admissibility}
%\leavevmode\\
%\newpage

\section{Estimated moments of the diameter of Zonotopes}
\import{Parties/}{7properties.tex}
\leavevmode\\

\section{Acknowledgments}
\import{Parties/}{8acknowledgment.tex}
\leavevmode\\

\bibliography{biblio}
\bibliographystyle{alphaurl}

\end{document}
